# Supplementary material for: MedLeak: Multimodal Medical Data Leakage in Secure Federated Learning with Crafted Models
Source: arXiv:2407.09972 source file (2025-06-29)
Supplement: Supplementary file 1 [file Appendix.tex]

%\section{Appendix}
